# Supplementary material for: A Completion-Aware Framework for Impactful Counterfactual Explainability in Graph Neural Networks
Source: arXiv:2606.22033 source file (2026-06-20)
Supplement: Supplementary file 2 [file macros.tex]

\newcommand{\TP}[1]{\textbf{Theodore Note: #1}}
\newcommand{\MV}[1]{\textbf{Myrto Note: #1}}

\newcommand{\cfx}{CFX } %abbreviation for counterfactual explanation

\newcommand{\LPframework}{DR-CFGNN }
